# Supplementary material for: Effect of second order piezoelectricity on excitonic structure of stress-tuned InGaAs/GaAs quantum dots
Source: arXiv:1805.06825 source file (2018-10-10)
Supplement: Supplementary file 1 [file dipole-paper-supplement.pdf]

# Supplemental Material for:

# Effect of second order piezoelectricity on excitonic structure of stress-tuned InGaAs/GaAs quantum dots

Petr Klenovský,[1,2,*] Petr Steindl,[1,2] Johannes Aberl,[3] Eugenio Zallo,[4,5] Rinaldo Trotta,[3,6] Armando Rastelli,[3] and Thomas Fromherz[3]

[1] *Department of Condensed Matter Physics, Faculty of Science, Masaryk University, Kotlářská 267/2, 61137 Brno, Czech Republic*
[2] *Central European Institute of Technology, Masaryk University, Kamenice 753/5, 62500 Brno, Czech Republic*
[3] *Institute of Semiconductor and Solid State Physics, Johannes Kepler University Linz, Altenbergerstraße 69, A-4040 Linz, Austria*
[4] *Institute for Integrative Nanosciences, IFW Dresden, Helmholtzstraße 20, D-01069 Dresden, Germany*
[5] *Paul-Drude-Institut für Festkörperelektronik, Hausvogteilplatz 5-7, 10117 Berlin, Germany*
[6] *Department of Physics, Sapienza University of Rome, Piazzale Aldo Moro 5, 00185 Rome, Italy*

(Dated: October 10, 2018)

## SI. DERIVATION OF THE RELATION BETWEEN IN-PLANE STRESS IN PRINCIPAL AND CARTESIAN COORDINATES

Any in-plane stress configuration can be described by three independent components of stress tensor ($\sigma_{xx}$, $\sigma_{yy}$, and $\sigma_{xy}$) or, equivalently, by two principal stresses $\sigma_{\rm max}$ and $\sigma_{\rm min}$ applied at an angle $\alpha$ with respect to the crystal axis. We now introduce the connection between the Cartesian and principal components.

We first rotate the basis of the stress components $\sigma_{xx}$, $\sigma_{yy}$ and $\sigma_{xy}$ by an angle $\theta$ to obtain components $\sigma'_{xx}$, $\sigma'_{yy}$ and $\sigma'_{xy}$ in the rotated basis which are related to the previous ones by

$$\sigma'_{xx} = \sigma_{xx}\cos^2\theta + \sigma_{yy}\sin^2\theta + 2\sigma_{xy}\sin\theta\cos\theta, \tag{1}$$

$$\sigma'_{yy} = \sigma_{xx}\sin^2\theta + \sigma_{yy}\cos^2\theta - 2\sigma_{xy}\sin\theta\cos\theta, \tag{2}$$

$$\sigma'_{xy} = (\sigma_{xx} - \sigma_{yy})\sin\theta\cos\theta + \sigma_{xy}\left(\cos^2\theta - \sin^2\theta\right). \tag{3}$$

Principal stress orientation can be then computed by setting $\sigma'_{xy} = 0$ in the last equation and solving

$$\sigma_{xx}\sin^2\theta + \sigma_{yy}\cos^2\theta - 2\sigma_{xy}\sin\theta\cos\theta = 0, \tag{4}$$

for $\theta$. The result is the equation giving the principal stress angle which we denote $\alpha$

$$\tan 2\alpha = \frac{2\sigma_{xy}}{\sigma_{xx} - \sigma_{yy}}. \tag{5}$$

Inserting $\alpha$ back into the Eqs. (1)–(3) we obtain the principal stress values $\sigma_{\rm max}$ and $\sigma_{\rm min}$

$$\sigma_{\rm max}, \sigma_{\rm min} = \frac{\sigma_{xx} + \sigma_{yy}}{2} \pm \sqrt{\left(\frac{\sigma_{xx} - \sigma_{yy}}{2}\right)^2 + \sigma_{xy}^2}. \tag{6}$$

We then express the sum and the difference of $\sigma_{\rm max}$ and $\sigma_{\rm min}$

$$\sigma_{\rm max} + \sigma_{\rm min} = \sigma_{xx} + \sigma_{yy}, \tag{7}$$

$$\sigma_{\rm max} - \sigma_{\rm min} = \sqrt{\left(\sigma_{xx} - \sigma_{yy}\right)^2 + 4\sigma_{xy}^2}. \tag{8}$$

If we now combine equations (6) with (8) we can write

$$\sigma_{xy} = \frac{1}{2}\left(\sigma_{\rm max} - \sigma_{\rm min}\right)\sin 2\alpha. \tag{9}$$

* klenovsky@physics.muni.cz

## SII. EXCITONIC FINE-STRUCTURE SPLITTING ENERGY AND DIPOLE AS FUNCTION OF $\sigma_{\rm max}+\sigma_{\rm min}$ FOR DIFFERENT DOT ELONGATION, HEIGHT, AND DIFFERENT PIEZOELECTRIC PARAMETERS

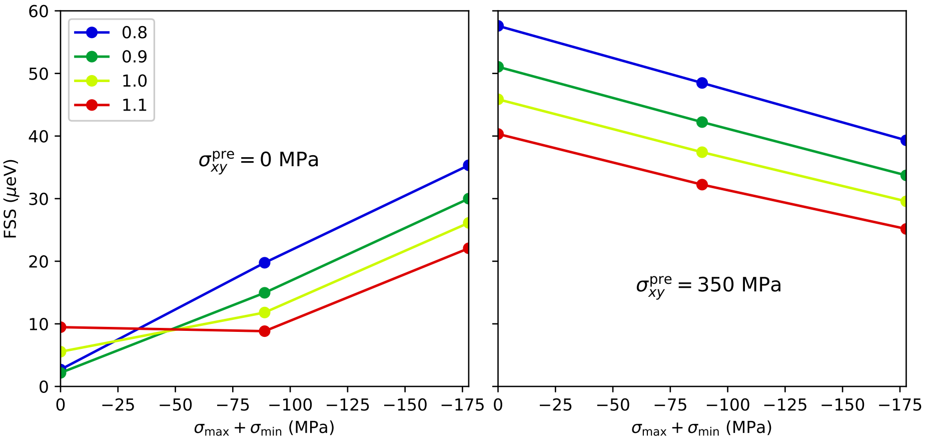


FIG. S1: Dependencies of FSS on $\sigma_{\rm max}+\sigma_{\rm min}$ for different QD elongations along [1-10] crystallographic axes, the values of that are given in inset of the left panel. The two panels show calculations for dots without prestress $\sigma_{xy}^{\rm pre}=0$ (left panel) and for $\sigma_{xy}^{\rm pre}=350$. Except of elongation and $\sigma_{xy}^{\rm pre}$ the simulated QDs had the same properties as $QD_2$. The dot elongation in $x-y$ plane was considered in such a way that the dot volume stayed the same for all cases.

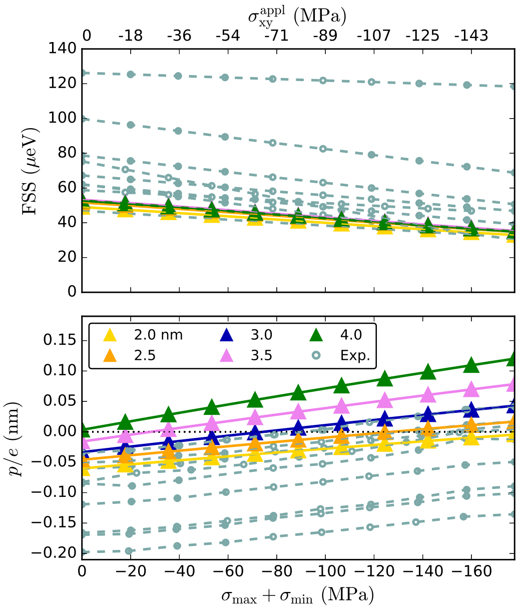


FIG. S2: Dependencies of FSS (top panel) and $p/e$ (bottom panel) on $\sigma_{\rm max}+\sigma_{\rm min}$ experimentally obtained from $\mu$PL measurements of nine InGaAs QDs [1] (broken curves) and that calculated for different values of dot height. Except of height the simulated QDs had the same properties as $QD_2$ including the value of $\sigma^{\rm pre}=350$ MPa. The letter $e$ denotes the elementary charge.

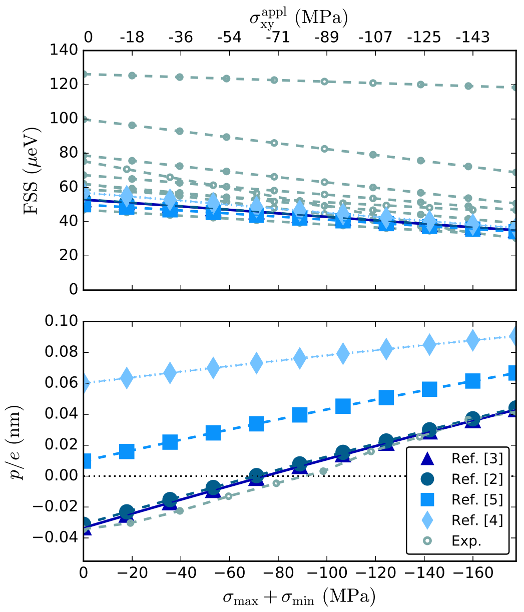


FIG. S3: Comparison of four sets of parameters of second order piezo, i.e. Refs. [2–5]. We show in top panel the dependence of emission energy FSS on applied stress $\sigma_{max} + \sigma_{min}$ and that for $p/e$ in lower panel. The experimental data from Ref. [1] are shown by broken gray curves.

## SIII. FITTED DEPENDENCIES OF $p/e$ ON $\sigma_{xy}^{appl}$ FOR EXPERIMENTAL DATA

The dependencies of $p/e$ on $\sigma_{xy}^{appl}$ were fitted by linear function $p/e = a \times \sigma_{xy}^{appl} + b$. The meaning of fitting parameters is $A^{QD} = a$ and $\sigma_{xy}^{pre} = b/a$.

TABLE I: Fitted dependencies of $p/e$ on $\sigma_{xy}^{appl}$ for experimental data shown in the main paper body.

| | a [nm/GaP] | b [nm] |
|---|---|---|
| Experiment | -0.51 ± 0.01 | -0.039 ± 0.001 |
| | -0.45 ± 0.01 | -0.055 ± 0.001 |
| | -0.45 ± 0.01 | -0.055 ± 0.001 |
| | -0.45 ± 0.01 | -0.055 ± 0.001 |
| | -0.45 ± 0.01 | -0.055 ± 0.001 |
| | -0.47 ± 0.01 | -0.066 ± 0.002 |
| | -0.55 ± 0.01 | -0.083 ± 0.002 |
| | -0.53 ± 0.01 | -0.094 ± 0.004 |
| | -0.46 ± 0.01 | -0.123 ± 0.001 |
| | -0.51 ± 0.01 | -0.171 ± 0.002 |
| | -0.46 ± 0.01 | -0.175 ± 0.002 |
| | -0.42 ± 0.01 | -0.202 ± 0.001 |

## SIV. MATERIAL PARAMETERS USED IN 8-BAND $\mathbf{k}\cdot\mathbf{p}$ CALCULATIONS OF INGAAS QDS

TABLE II: Values of the material parameters used in 8 $\mathbf{k}\cdot\mathbf{p}$ calculations. The references from which the parameters were taken are identified in the last column. The parameters $\gamma_1$, $\gamma_2$, and $\gamma_3$ are the Luttinger parameters [6]. Note, that all parameters are spatially dependent.

| Parameter | Description | Unit | InAs | GaAs | Ref. |
|---|---|---|---|---|---|
| $a$ | lattice constant | Å | 6.0583 | 5.6533 | [7] |
| $a_{\mathrm{exp}}$ | lattice thermal expansion coefficient | Å/K | $2.74\times10^{-5}$ | $3.88\times10^{-5}$ | [7] |
| $C_{11}$ | elastic constant | GPa | 83.29 | 122.1 | [7] |
| $C_{12}$ | elastic constant | GPa | 45.26 | 56.6 | [7] |
| $C_{44}$ | elastic constant | GPa | 39.59 | 60.0 | [7] |
| $E_0$ | bandgap energy | eV | 0.417 | 1.519 | [7] |
| $\varepsilon_{\mathrm{r}}$ | static dielectric constant | - | 15.15 | 12.93 | [8] |
| $\alpha$ | Varshni parameter [9] | eV/K | $0.276\times10^{-3}$ | $0.541\times10^{-3}$ | [7] |
| $\beta$ | Varshni parameter [9] | K | 93 | 204 | [7] |
| $E_{\mathrm{v}}$ | valence band offset | eV | 1.390 | 1.346 | [10] |
| $\Delta_0$ | spin-orbit split-off energy | eV | 0.390 | 0.341 | [7] |
| $a_{\mathrm{c}}$ | absolute deformation potential for conduction band | eV | $-6.66$ | $-9.36$ | [10] |
| $a_{\mathrm{v}}$ | absolute deformation potential for valence band | eV | $-1.00$ | $-1.21$ | [10] |
| $a_{\mathrm{ub}}$ | uniaxial shear deformation potential of the valence bands in the [100] direction | eV | $-1.8$ | $-2.0$ | [7] |
| $a_{\mathrm{ud}}$ | uniaxial shear deformation potential of the valence bands in the [111] direction | eV | $-3.6$ | $-4.8$ | [7] |
| $S$ | electron effective mass parameter | - | $-4.80$ | $-2.88$ | [7] |
| $E_{\mathrm{p}}$ | Kane's momentum matrix element | eV | 21.5 | 28.8 | [7] |
| $L$ | Dresselhaus parameter [11]; $L=-\gamma_1-4\gamma_2-1$ | $\hbar^2/2m_0$ | $-15.695$ | 1.420 | [7] |
| $M$ | Dresselhaus parameter [11]; $M=2\gamma_2-\gamma_1-1$ | $\hbar^2/2m_0$ | $-4.0$ | $-3.9$ | [7] |
| $N$ | Dresselhaus parameter [11]; $N=-6\gamma_3$ | $\hbar^2/2m_0$ | $-15.895$ | 0.056 | [7] |

TABLE III: Composition dependence of the input parameters of $\mathrm{In_xGa_{1-x}As}$ used in the calculations. The labeling of parameters is defined in Tab. II. The references from which parameters were taken are identified in the last column. Those parameters whose reference is missing were provided by the parameter library of nextnano3 [12].

| Parameter | Unit | $\mathrm{In_xGa_{1-x}As}$ | Ref. |
|---|---|---|---|
| $a$ | Å | linear | |
| $a_{\mathrm{exp}}$ | Å/K | linear | |
| $C_{11}$ | GPa | linear | |
| $C_{12}$ | GPa | linear | |
| $C_{44}$ | GPa | linear | |
| $E_0$ | eV | $0.417x+1.519(1-x)-0.477x(1-x)$ | [7] |
| $\varepsilon_{\mathrm{r}}$ | - | linear | |
| $\alpha$ | eV/K | linear | |
| $\beta$ | K | linear | |
| $E_{\mathrm{v}}$ | eV | $1.39x+1.346(1-x)+0.38x(1-x)$ | [7] |
| $\Delta_0$ | eV | $0.39x+0.341(1-x)-0.15x(1-x)$ | [7] |
| $a_{\mathrm{c}}$ | eV | $-6.66x-9.36(1-x)-2.61x(1-x)$ | [7] |
| $a_{\mathrm{v}}$ | eV | linear | |
| $a_{\mathrm{ub}}$ | eV | linear | |
| $a_{\mathrm{ud}}$ | eV | linear | |
| $S$ | - | $-4.80x-2.88(1-x)-3.54x(1-x)$ | [7] |
| $E_{\mathrm{p}}$ | eV | $21.5x+28.8(1-x)+1.48x(1-x)$ | [7] |
| $L$ | $\hbar^2/2m_0$ | $-15.695x+1.420(1-x)+25.063x(1-x)$ | [7] |
| $M$ | $\hbar^2/2m_0$ | $-4.0x-3.86(1-x)+1.141x(1-x)$ | [7] |
| $N$ | $\hbar^2/2m_0$ | $-15.895x+0.056(1-x)+26.809x(1-x)$ | [7] |

[1] J. Aberl, P. Klenovský, J. S. Wildmann, J. Martín-Sánchez, T. Fromherz, E. Zallo, J. Humlíček, A. Rastelli, and R. Trotta, Phys. Rev. B **70**, 201308 (2017), URL `http://link.aps.org/doi/10.1103/PhysRevB.70.201308`.
[2] G. Bester, X. Wu, D. Vanderbilt, and A. Zunger, Phys. Rev. Lett. **96**, 187602 (2006), URL `http://link.aps.org/doi/10.1103/PhysRevLett.96.187602`.
[3] A. Beya-Wakata, P. Y. Prodhomme, and G. Bester, Physical Review B **84**, 195207 (2011).
[4] G. Tse, J. Pal, U. Monteverde, R. Garg, V. Haxha, M. A. Migliorato, and S. Tomic, Journal of Applied Physics **114**, 073515 (2013).
[5] M. A. Caro, S. Schulz, and E. P. O'Reilly, Phys. Rev. B **91**, 075203 (2015), URL `http://link.aps.org/doi/10.1103/PhysRevB.91.075203`.
[6] J. M. Luttinger, Physical Review **102**, 1030 (1956).
[7] I. Vurgaftman, J. Meyer, and L. Ram-Mohan, J. Appl. Phys. **89**, 5815 (2001).
[8] Landolt–Börnstein, *Numerical data and functional relationships in science and technology*, new series, Vol. III/17a (Springer, Berlin, 1982).
[9] Y. Varshni, Physica **34**, 149 (1967).
[10] S. Wei and A. Zunger, Appl. Phys. Lett. **72**, 2011 (1998).
[11] G. Dresselhaus, A. Kip, and C. Kittel, Phys. Rev. **98**, 368 (1955).
[12] S. Birner, T. Zibold, T. Andlauer, T. Kubis, M. Sabathil, A. Trellakis, and P. Vogl, IEEE Trans. El. Dev. **54**, 2137 (2007).
